# Supplementary material for: Is Decentralized Finance Actually Decentralized? An Interdisciplinary Framework Integrating Network Theory, Agent-Based Simulation, and Longitudinal Evidence from Aave, GHO Issuance, and Cross-Chain Expansion
Source: arXiv:2206.08401 source file (2026-10-05)
Supplement: Supplementary file 1 [file evidence_status_ledger.tex]

\section{Evidence-status ledger}\label{app:evidence-ledger}

\begin{table*}[!ht]
\centering
\caption{Release-level evidence and claim status.}
\label{tab:evidence-status-ledger}
\AVTableSetup
\begin{tabularx}{0.99\textwidth}{p{0.13\textwidth}p{0.23\textwidth}Xp{0.18\textwidth}}
\toprule
\AVTableHeader
\textbf{Release} & \textbf{Verified object} & \textbf{Supported use} & \textbf{Hard stop} \\
\midrule
\texttt{real\_v1} & Recovery boundary and legacy Ethereum source & Method provenance & Not the governed longitudinal panel \\
\texttt{real\_v2} & 118,806 Ethereum Pool events & Address-level measurement and action composition & No actor or causal result \\
\texttt{real\_v3} & Historical code and 10 curated labels & Contract/address-type sensitivity & Economic-actor coverage 0\% \\
\texttt{real\_v4} & Position-holder panel and period HHI bounds & Pooled address HHI and period-specific actor bounds & Change envelope is not a sharp joint set \\
\texttt{real\_v5} & Ethereum--Arbitrum weekly panels and topology & Longitudinal descriptive and structural evidence & Clocks differ; no route table or ATT \\
\texttt{real\_v6} & Audited Arbitrum--Gnosis common-calendar panel & Reproducible comparative longitudinal analysis and diagnostics & Differential pre-path; comparison-driven movement; no treatment effect \\
\texttt{causal\_v2} & Corrected multichain collector and tests & Future acquisition pipeline & Governed multichain ATT not produced \\
\texttt{bridge\_v2} & Route schema and planned diagnostics & Future infrastructure design & Verified route-event panel absent \\
Subgraph & Pinned reconciliation protocol & Future independent validation & Not executed; supports no current result \\
\bottomrule
\end{tabularx}
\end{table*}

The machine-readable ledger records the archived acquisition run and digest, compact-output paths, acquisition and analysis pipeline versions, and the boolean claim gates. A release may contain conventional comparative coefficients while leaving the causal estimand unidentified. This is intentional: computational completion and identification are separate states.
