# Supplementary material for: Is Decentralized Finance Actually Decentralized? An Interdisciplinary Framework Integrating Network Theory, Agent-Based Simulation, and Longitudinal Evidence from Aave, GHO Issuance, and Cross-Chain Expansion
Source: arXiv:2206.08401 source file (2026-10-05)
Supplement: Supplementary file 7 [file future_causal_infrastructure_extensions.tex]

\section{Future systemic and agent-mediated extensions}\label{app:future-extensions}\label{app:future-systemic}

\subsection{Corrected multichain outcome panels}
The multichain collection procedure maps Supply and Borrow \texttt{onBehalfOf} to indexed topic 2 rather than the referral-code field at topic 3, and it rejects invalid zero-address position holders. Existing compact Avalanche, Metis, and zkSync Era files were created before that correction and cannot be repaired because they omit raw topics and data. They remain acquisition-audit records, not outcome panels. Every affected deployment must be collected again and pass ABI-semantic, window-continuity, duplicate-key, provider, and reproducibility checks before estimation.

\subsection{Staggered causal design}
The intended multichain extension uses verified GHO reserve activations, common outcome semantics, and not-yet-treated deployments on overlapping calendars. It will estimate group-time, interaction-weighted, or imputation event-study effects only after sufficient pre-treatment support, explicit anticipation windows, clean event-study leads, chain-level inference, alternative windows, and leave-one-chain-out diagnostics meet the stated criteria \cite{callaway2021difference,sun2021estimating,borusyak2024revisiting}. Treatment-timing decompositions will be reported where conventional two-way fixed-effects summaries could combine heterogeneous cohort comparisons \cite{goodmanbacon2021difference}. The estimand applies to the admitted data-complete deployments and does not automatically generalize to every Aave deployment. Synthetic control or synthetic difference-in-differences remains a proposed robustness design requiring comparison fit, predictor balance, and placebo evidence.

\begin{table*}[!ht]
\centering
\caption{Future multi-chain identification roadmap. This is a conceptual research-design table; it reports no estimates from the present study.}
\label{tab:future-identification-roadmap}
\AVTableSetup
\begin{tabularx}{0.99\textwidth}{P{0.15\textwidth}P{0.17\textwidth}P{0.17\textwidth}YP{0.20\textwidth}}
\toprule
\AVTableHeader
\textbf{Future design} & \textbf{Required data} & \textbf{Comparison strategy} & \textbf{Core identifying requirements} & \textbf{Candidate method} \\
\midrule
Repeated GHO expansions & Multiple validated destination-chain panels & Not-yet-treated deployments & Comparable semantics, conditional parallel trends, bounded anticipation & Group-time or interaction-weighted DiD \\
Synthetic comparison & Larger verified comparison pool & Pre-specified weighted deployments & Stable pre-event fit, predictor balance, placebo support & Synthetic control or synthetic DiD \\
Chain event study & Multiple activation cohorts and dates & Cohort-specific comparisons & No hidden anticipation, valid cohort support, chain-level inference & Imputation event study \\
Infrastructure adoption & Verified route and dependency events & Routes or chains without the change & No concurrent differential route shock; stable measurement & DiD or controlled ITS \\
Agentic experiment & Validated adaptive-agent environment & Randomized simulation conditions & Model-valid assignment, repeated seeds, provider dependence disclosed & Simulation experiment \\
\bottomrule
\end{tabularx}
\end{table*}

\begin{table*}[!ht]
\centering
\caption{Evidence required before stronger causal claims. This is a conceptual requirements table, not an empirical-results table.}
\label{tab:future-causal-requirements}
\AVTableSetup
\begin{tabularx}{0.99\textwidth}{P{0.19\textwidth}P{0.21\textwidth}YP{0.21\textwidth}}
\toprule
\AVTableHeader
\textbf{Prospective claim} & \textbf{Additional evidence} & \textbf{Falsification and sensitivity checks} & \textbf{Appropriate inference} \\
\midrule
GHO changes participation & Several same-semantic chain panels and verified activation clocks & Pre-paths, anticipation, concurrent-event ledger, leave-one-chain-out & Chain- or cohort-level design-based inference \\
GHO changes concentration & Address-role outcomes plus actor-linkage sensitivity & Outcome definitions, reserve/action decompositions, bounded trend departures & Multi-chain DiD or validated synthetic comparison \\
Expansion improves resilience & Route occurrences, capacities, shared components, and substitution rules & Route removals, correlated failures, rerouting, recovery scenarios & Design-specific uncertainty plus calibrated stress tests \\
Automation decentralizes decisions & Delegation, authorization, agent, provider, and beneficiary provenance & Shared-model ablations, synchronization tests, human-confirmation sensitivity & Experimental or validated longitudinal design \\
\bottomrule
\end{tabularx}
\end{table*}

\subsection{Economic-actor resolution}
Actor identification will accept only dated primary-source controller evidence with validity intervals and a documented correction history. Exchange, multisignature, smart-wallet, router, bridge, and protocol labels may improve coverage, but bytecode, co-timing, shared counterparties, or behavioral similarity alone will not create must-links. When coverage remains incomplete, actor-level concentration will continue to be reported as an identified set.

\subsection{Route and infrastructure evidence}
Infrastructure analysis requires verified occurrence records linking chain, route, source and destination contracts, facilitator, messaging provider, asset, transaction, amount, and time. Once that layer exists, the analysis can estimate route HHI, facilitator concentration, disjoint paths, minimum cuts, removal loss, oracle dependence, and common-route stress. A governance configuration transaction or a Pool event does not by itself prove that a route carried the measured economic activity. Until route-event coverage and counterfactual reassignment rules are assessed, infrastructure results remain unavailable.



\subsection{Dynamic systemic and agent-mediated research agenda}

This appendix separates implementable research designs from results established in the present study. Every item below is prospective. None changes the evidence status of the four measured dimensions, identifies an average treatment effect, converts addresses into economic actors, or establishes the presence of autonomous agents in the analyzed Aave events.

\subsection{A dynamic heterogeneous multilayer representation}

A future protocol system at time \(t\) can be represented as
\[
\mathcal{G}_t=\left(
V_t,
E_t^{\mathrm{lending}},
E_t^{\mathrm{GHO}},
E_t^{\mathrm{transfer}},
E_t^{\mathrm{bridge}},
E_t^{\mathrm{governance}},
E_t^{\mathrm{infrastructure}}
\right).
\]
The layers encode functional, contractual, or institutional relations. Ethereum, Arbitrum, and other blockchains may define chain-specific partitions within those layers, but they are not geographical regions. Nodes may represent addresses or evidence-supported entities, contracts, assets, facilitators, bridges, or infrastructure providers. Identity links across layers must retain provenance and uncertainty rather than silently treating heuristic clusters as known actors.

Memory-aware community analysis can identify persistent groups and role changes \cite{clemente2024memory}. Higher-order events can retain joint relations among users, contracts, assets, and infrastructure rather than reducing every event to pairwise projections \cite{iacopini2024temporal}; the choice between hypergraph and simplicial representations must be justified because it can change the implied dynamics \cite{zhang2023higherorder}. Temporal aggregation can likewise be selected according to its dynamical consequences \cite{allen2024compressing}. These methods motivate future analysis but do not retroactively alter the weekly pairwise networks used in the paper.

\input{figures/fig21_future_systemic_decentralization}

\subsection{Staged analytical roadmap}

\begin{table}[!htbp]
\centering
\caption{Prospective roadmap from observed protocol networks to systemic and agent-mediated decentralization. Each stage adds data or assumptions and therefore requires a new validation gate.}
\label{tab:future-systemic-roadmap}
\begin{tabularx}{\textwidth}{>{\raggedright\arraybackslash}p{0.07\textwidth}>{\raggedright\arraybackslash}p{0.19\textwidth}>{\raggedright\arraybackslash}p{0.25\textwidth}>{\raggedright\arraybackslash}X}
\toprule
Stage & Extension & Advancement & Required evidence or validation \\
\midrule
1 & Temporal multilayer construction & Links lending, GHO, transfer, bridge, governance, and infrastructure relations & Verified contracts, event schemas, cross-chain message matching, and layer-specific completeness checks \\
2 & Probabilistic entity resolution & Distinguishes address growth from economic-actor growth & Primary-source ownership links, sensitivity bounds, and explicit uncertainty propagation \\
3 & Higher-order event representation & Preserves joint operational groups instead of only pairwise projections & Event-level participant roles and theoretical justification for hypergraph or simplicial encoding \\
4 & Memory-aware roles & Measures persistent cores and peripheral--broker--core transitions & Stable observation windows, temporal-resolution sensitivity, and out-of-sample role stability \\
5 & Infrastructure stress tests & Estimates direct and cascading dependency losses & Route tables, substitution rules, calibrated capacities, and failure scenarios grounded in documented infrastructure \\
6 & Agentic behavioral simulation & Adds heterogeneous memory, information, tools, and adaptive strategies & Behavioral benchmarks, controlled ablations, repeated seeds, model/provider disclosure, and validation against observed responses \\
7 & Verified delegation layer & Measures agency-and-delegation concentration \(\mathcal D_t\) & Agent labels, authorization records, wallet permissions, intent attestations, execution traces, and beneficiary evidence \\
\bottomrule
\end{tabularx}
\end{table}

The order is substantive. Later stages should not be presented as more realistic merely because they are more complex. Each is warranted only when its additional objects are identifiable and its behavior can be validated. Graph neural networks could eventually assist prediction of role transitions or distress, but interpretable construction, entity uncertainty, temporal persistence, and resilience testing come first.

\subsection{Agentic simulation as a methodological extension}

The present simulation solves a transparent network game under stated rules. A future agentic simulation could add heterogeneous objectives, risk preferences, memory, bounded reasoning, differentiated tools and information, entry and exit, and adaptive responses to issuance, bridge costs, and liquidity conditions. It could examine whether autonomous execution accelerates liquidity formation, discovers cross-chain arbitrage, synchronizes withdrawals or liquidations, or amplifies shocks through common infrastructure. The language-model agents in EconAgent demonstrate one route to heterogeneous multi-period economic simulation \cite{li2024econagent}; they do not validate a DeFi calibration.

A responsible design would retain the current theorem-based simulation as a baseline, add behavioral agents in controlled increments, compare identical environments across agent architectures, and report model/provider dependence as part of the experimental treatment. Repeated strategies produced by one shared foundation model are not independent evidence merely because they control different wallets. Validation should compare simulated action distributions, timing, transitions, and shock responses with held-out protocol behavior, while documenting where no credible observational target exists.

\subsection{Agency-and-delegation concentration}

The prospective fifth dimension asks how concentrated effective decision-making is across the chain of principals, decision systems, executors, and beneficiaries. Let an independently verified delegation graph \(D_t\) link these roles. Candidate summaries include principal HHI across agent-operated wallets, agent-provider or strategy-provider HHI, the number of principals depending on one model or execution service, synchronization of actions after shocks, and the share of autonomous versus human-confirmed transactions.

These measures require a stronger evidentiary basis than transaction records alone. The qualitative typology of crypto-related agents in \citet{ante2025autonomous} motivates hypotheses about possible roles but remains exploratory evidence and does not label this study's transactions. Accordingly, \(\mathcal D_t\) must remain outside the current empirical vector until delegation, authorization, execution, and beneficiary links are independently verified.

\subsection{Causal and resilience designs}

Future causal work can build chain--reserve--action panels with multiple adoption cohorts, stable pre-event support, transparent comparison selection, and estimators appropriate to staggered timing. Network-aware designs should also allow one actor's exposure to affect connected actors, because conventional no-interference assumptions may be implausible in lending and liquidation networks. Route resilience requires a separate design: direct removal identifies immediate reachability loss, while cascading analysis requires behavioral substitution, capacity constraints, and cross-layer coupling. The higher-order multilayer framework of \citet{nicoletti2024information} is useful for formulating such propagation, but empirical calibration remains a distinct task.

The resulting progression is:
\[
\begin{aligned}
\text{measure observed decentralization}
&\rightarrow \text{model cross-layer evolution}\\
&\rightarrow \text{simulate dependency failures}\\
&\rightarrow \text{evaluate delegated decision concentration}.
\end{aligned}
\]
The governing question is whether protocol expansion distributes economic participation and control or instead relocates concentration across actors, layers, infrastructure, and decision providers.
