# Supplementary material for: Is Decentralized Finance Actually Decentralized? An Interdisciplinary Framework Integrating Network Theory, Agent-Based Simulation, and Longitudinal Evidence from Aave, GHO Issuance, and Cross-Chain Expansion
Source: arXiv:2206.08401 source file (2026-10-05)
Supplement: Supplementary file 8 [file literature_coding_audit.tex]

\section{Fixed-corpus literature coding audit}\label{app:literature-coding}

The main-text literature synthesis is claim-led and includes both foundational and recent boundary-setting work. The supplementary coding audit below serves a narrower reproducibility purpose. It preserves the fixed 18-work ledger developed for the earlier method--domain--evidence classification, so every ribbon can be traced to a released paper-level assignment without silently recoding the corpus during the present narrative revision. The audit is therefore not an exhaustive literature review and should not be used to infer the relative size or importance of a field.

\input{figures/fig02c_literature_method_evidence}
